# Supplementary material for: Predicting Flat-Fading Channels via Meta-Learned Closed-Form Linear Filters and Equilibrium Propagation
Source: arXiv:2110.00414 source file (2022-03-06)
Supplement: Supplementary file 1 [file appendix.tex]

\section{SCM-Based Channel Model}
\label{app:1}
In Sec.~\ref{sec:exp_standard_off} and Sec.~\ref{sec:exp_standard_on}, we assume a frequency-flat channel that is obtained as a special case of the standard multipath spatial channel models \cite{3gpp_tr_901}. Accordingly, the channel $h_{l,f}$ can be expressed as the combination of $d_{total}$ paths as
\begin{align}
    h_{l,f} = \sum_{d=1}^{d_{total}} \sqrt{\Omega_{d,f}}A_{d,l,f}.
    \label{eq:multivariate_channel_model}
\end{align}
In \eqref{eq:multivariate_channel_model}, the contribution of the $d$-th path depends on the average power $\Omega_{d,f}$, which is constant within one frame, and on the complex fading gain $A_{d,l,f}$. We assume that the channel coherence time is larger than the slot duration, so that the fading amplitude $A_{d,l,f}$ is constant within one slot and varies accordingly to a stationary process along the slots of one frame \cite{cicerone2006channel}.
The complex gain $A_{d,l,f}$ is modeled as
\begin{align}
A_{d,l,f} =& \mathbf{F}_{rx}(\theta_{d,f,ZOA}, \phi_{d,f,AOA})^T \cdot \mathbf{M}_{d,f}  \\&\cdot\mathbf{F}_{tx}( \theta_{d,f,ZOD},\phi_{d,f,AOD}) \\&\cdot \exp{\left(-\frac{j2\pi \delta_{d,f}}{\lambda_0}\right)} \cdot \exp{\left( -jw_{d,f} t_l\right)},
\label{eq:3gpp_channel_model}
\end{align}
where $\mathbf{F}_{rx}(\cdot,\cdot)$ and $\mathbf{F}_{tx}(\cdot,\cdot)$ are the $2 \times 1$ field patterns of the receive and transmit antenna; $\theta_{d,f,ZOA}$, $\phi_{d,f,AOA}$,  $\theta_{d,f,ZOD}$, $\phi_{d,f,AOD}$ are the zenith angle of arrival (ZOA), azimuth angle of arrival (AOA), zenith angle of departure (ZOD), azimuth angle of departure (AOD) (in $^\circ$); $\lambda_0$ is the wavelength (in $\text{m}$) of the carrier frequency; $\delta_{d,f}$ is the length of the path (in $\text{m}$); $w_{d,f} \in [0,2\pi v_\text{max}/\lambda_0]$ is the normalized Doppler frequency (in $\text{rad}/\text{s}$) with maximum user speed $v_\text{max}$ (in $\text{m}/\text{s}$); $t_l$ is the starting wall-clock time of the $l$-th slot (in $\text{s})$; and $M_{d,f}$ is the polarization coupling matrix defined as
\begin{align}
    \mathbf{M}_{d,f} = \left(\begin{array}{ll} \quad \quad \exp{\left(j\Phi^{\theta \theta}_{d,f}\right)} \quad\quad\quad\quad \sqrt{1/\kappa_{d,f}}\cdot \exp{\left( j \Phi_{{d,f}}^{\theta \phi} \right)} \\ \sqrt{1/\kappa_{{d,f}}}\cdot \exp{\left( j \Phi_{{d,f}}^{\phi \theta} \right)}\quad\quad\quad\quad \exp{\left(j\Phi^{\phi \phi}_{d,f}\right)} \end{array} \right),
\end{align}
with random initial phase $\Phi_{d,f}^{(\cdot, \cdot)} \sim U(-\pi,\pi)$ and log-normal distributed cross polarization power ratio (XPR) $\kappa_{d,f}>0$. The long-term features given by ZOA, AOA, ZOD, AOD do not change within a frame $f$. By \eqref{eq:multivariate_channel_model}, the Doppler spectrum of the channel $h_{l,f}$ across the slots $l=1,2,\ldots$ of frame $f$ depends on the Doppler frequency $w_{d,f}$ and on the distribution of the path lengths and angles. These multipath parameters can change in arbitrary ways across the frames.

\section{Online Meta-Learning via Implicit Gradient}
\label{app:2}
Here we introduce an alternative approach to compute the gradient of the objective \eqref{eq:obj_for_gradient_methods} via the implicit gradient theorem \cite{rajeswaran2019meta, lorraine2020optimizing}. From our experiments, the EP-based approach described in Sec.~\ref{sec:EP-online} tends to have comparable performance and is simpler to implement, but the implicit gradient method is conceptually valid and may be advantageous in different settings \cite{rajeswaran2019meta, lorraine2020optimizing}. 

From the chain rule, the gradient of the objective in \eqref{eq:obj_for_gradient_methods} can be written as
\begin{align}
    \nabla_{\bar{v}}L_f^\text{outer}\left(v_\lambda^*(\mathcal{Z}_f^\text{tr}|\bar{v})\right) = \nabla_{\bar{v}}v_\lambda^*(\mathcal{Z}_f^\text{tr}|\bar{v}) \cdot  \nabla_{v_\lambda^*(\mathcal{Z}_f^\text{tr}|\bar{v})} L_f^\text{outer}(v_\lambda^*(\mathcal{Z}_f^\text{tr}|\bar{v})).
    \label{eq:total_grad_scalar}
\end{align}
By the implicit function theorem \cite{rajeswaran2019meta, lorraine2020optimizing}, the Jacobian $\nabla_{\bar{v}}v_\lambda^*(\mathcal{Z}_f^\text{tr}|\bar{v})$ can be computed 
\begin{align}
    \nabla_{\bar{v}}v_\lambda^*(\mathcal{Z}_f^\text{tr}|\bar{v}) = \left(I+\frac{1}{2\lambda} \nabla^2_{v}L_f(v)\right)^{-1} \bigg|_{v = v_\lambda^*(\mathcal{Z}_f^\text{tr}|\bar{v})}.
    \label{eq:implicit_inverse}
\end{align}
Plugging \eqref{eq:implicit_inverse} into \eqref{eq:total_grad_scalar} finally yields the gradient
\begin{align}
    \nonumber
    \nabla_{\bar{v}}L_f^\text{outer}&\left(v_\lambda^*(\mathcal{Z}_f^\text{tr}|\bar{v})\right) \\\nonumber= \Big(I+&\frac{1}{2\lambda} \nabla^2_{v}L_f(v)\Big)^{-1} \bigg|_{v = v_\lambda^*(\mathcal{Z}_f^\text{tr}|\bar{v})} \\\nonumber&\cdot \nabla_{v_\lambda^*(\mathcal{Z}_f^\text{tr}|\bar{v})} L_f^\text{outer}(v_\lambda^*(\mathcal{Z}_f^\text{tr}|\bar{v})) \\\nonumber
    = \Big( \frac{1}{\lambda}& (X_f^\text{tr})^\dagger X_f^\text{tr} + I \Big)^{-1} \\&\cdot 2(X_f^\text{te})^\dagger\left( X_f^\text{te} v^*_\lambda(\mathcal{Z}_f^\text{tr}|\bar{v}) - y_f^\text{te} \right).
    \label{eq:implicit_meta_grad}
\end{align}
Note that, unlike the EP-based gradient estimate \eqref{eq:EP_grad_actual}, the gradient \eqref{eq:implicit_meta_grad} is exact and it requires a matrix inversion of the same complexity as the closed-form solution \eqref{eq:closed_from_sol_meta_scalar} (with some rearrangement, \eqref{eq:implicit_meta_grad} is equivalent to the gradient that can be obtained from the closed-form solution \eqref{eq:closed_from_sol_meta_scalar}, i.e., $2(\tilde{X}_f^\text{te})^\dagger(\tilde{X}_f^\text{te}\bar{v}-\tilde{y}_f^\text{te})$).
